# Supplementary material for: Learning-to-Fly: Learning-based Collision Avoidance for Scalable Urban Air Mobility
Source: arXiv:2006.13267 source file (2020-06-23)
Supplement: Supplementary file 1 [file appendix.tex]

%Appendix
%\clearpage
%\section{Appendix}
%\appendix
\section*{APPENDIX}
\label{sec:Appendix}

\subsection{A greedy algorithm for conflict resolution}
\label{sec:greedy_alg}

For a horizon length of $N$ steps, there are $6^{N}$ possible selections for the deconfliction constraints $H^i_k, \, g^i_k$ (6 at each time step in the horizon). The centralized MILP formulation picks which constraint to use by activating the corresponding binary variable \eqref{eq:CentralMILP}. For CA-MPC, we need a decision making algorithm to pick these constraints as there are no binary variables in the CA-MPC formulations \eqref{eq:drone1mpc}, \eqref{eq:drone2mpc}. 

The following is a greedy approach to this:

\begin{algorithm}
 \KwData{Pre-planned trajectories: $\mathbf{x_1}, \, \mathbf{x_2}$, a preset maneuver: $\text{preset} \in \{1,\dotsc,6\}$}
 \KwResult{$d_k \in \{1,\dotsc,6\}\, \forall k=\{0,\dotsc, N+1\}$ for conflict resolution maneuvers $H^{d_k},\, g^{d_k}$}
 initialization k=0, \; \\
 \While{$k \leq N+1$}{
 \For{$i=\{1,\dotsc,6\}$}
 {$r^{i}_k = g^i - H^i C(x_{1,k}-x_{2,k})$
 }
 %$i[k] = \text{argmax}_i\, (g_i - H_i (x_1[k]-x_2[k]))$ \\
 \eIf{$\exists i|r^i_k \geq 0 $}{
 $d_k = \text{argmax}_i\, r_{i}[k]$
 }
 {$d_k = \text{preset}$
 }
 k = k+1
%  read current\;
%  \eIf{understand}{
%   go to next section\;
%   current section becomes this one\;
%   }{
%   go back to the beginning of current section\;
%  }
 }
 \caption{Greedy conflict resolution}
 \label{alg:greedy}
\end{algorithm}

Algorithm \ref{alg:greedy}, for time steps $k$ such that there is no 
conflict, selects the direction (or side of the hypercube 
\eqref{eq:noconf}) where there is the most separation between the 
UAS. For the time steps where there is a conflict, it picks a 
pre-defined maneuver.
\subsection{Case Study: Equipment Surveillance Scenario}
\label{sec:rural_case}

\begin{figure}[tb]
	\begin{center}
		\includegraphics[width=0.49\textwidth]{figures/rural_out}
	\end{center}
	{\footnotesize
		\caption{\small Trajectories for 4 UAS tasked with flying over the
			pumpjacks by reaching the all green-colored goal set 
			within 10 minutes, while avoiding the all black-colored 
			obstacles (the
			pumpjacks themselves).}
		\label{fig:rural}}
\end{figure}

The equipment surveillance scenario taken 
from~\cite{wargo2014unmanned} outlines a low-altitude mission profile 
for four UAS operating within a sparsely populated area. The airspace 
setting is depicted in a Figure~\ref{fig:rural}. This scenario can 
serve as a template
for other rural use cases for UAS such as end-point package
deliveries and wildfire management.

The mission for each UAS $j\in\{1,\ldots,4\}$
is formalized in STL as following:
\begin{equation}
\label{eq:rural_d}
\begin{aligned}
\varphi_j =  \bigwedge_{n=1}^5
\eventually_{[0,10]} (p_j \in \text{Zone}_n)
&\land \eventually_{[9,10]} (p_j \in \text{EndZone}_j) \\
&\land\always_{[0,10]} \neg (p_j \in \text{Unsafe})
\end{aligned}
\end{equation}
where 
$T=10$m is the maximum allowable flight time
allocated to the mission, $\text{Zone}_n$ denotes the airspace region 
directly above each
of the five pumpjacks, $\text{Unsafe}$ denotes the no-fly zones within
the mission environment and $\text{EndZone}_j$ defines the region 
signifying the end of the UAS mission.

Table~\ref{tbl:runtimes_rural} shows the computation times 
for solving the planning problem in a centralized manner versus 
solving for each 
UAS $j$ and its specification $\varphi_j$ separately.

\begin{table}[]
	
	\caption{Computation times for the centralized versus individual 
		UAS planning
	}
	\label{tbl:runtimes_rural}
	
	\centering
	\begin{tabular}{c|c|c|c|c|c|}
		\cline{2-6}
		\multicolumn{1}{l|}{}                   & 
		\textbf{Centralized} & 
		\multicolumn{4}{c|}{\textbf{Independent 
				planning}}                   
		\\ \cline{2-6} 
		& \textbf{4 UAS}    & \textbf{UAS 1} & \textbf{UAS 2} & 
		\textbf{UAS 3} & \textbf{UAS 4} \\ \cline{2-6} 
		\hline\hline
		\multicolumn{1}{|c|}{\textbf{Mean (s)}} & 
		81.918               & 15.596          & 
		17.444            & 
		17.553           &   16.128        \\ \hline
		\multicolumn{1}{|c|}{\textbf{SD (s)}} & 
		27.215           & 6.257        & 
		7.404            & 
		6.912           &  6.764        \\ \hline
	\end{tabular}
\end{table}

\subsection{Separation Profile}
\label{sec:separation}

Figure~\ref{fig:sep_profile} depicts the separation profile over 
time before and after L2F for one of 10K minimum-jerk random 
trajectories described in the Section~\ref{sec:exp_setup}.

\begin{figure}[t]
	\begin{center}
		\includegraphics[width=0.45\textwidth]{figures/t3.png}
	\end{center}
	{\footnotesize
		\caption{\small The separation profile before and after L2F 
		for one of the minimum-jerk random trajectories described in 
		the Section~\ref{sec:exp_setup}.}
		\label{fig:sep_profile}}
\end{figure}

\subsection{Brief discussion on minimum separation and CA-MPC 
objective value}
\label{sec:slackbad}

\begin{figure}
	\begin{subfigure}[b]{0.4\columnwidth}
		\includegraphics[width=1.25\linewidth]{figures/slack_distance153.png}
		%\caption{Picture 1}
		\label{fig:1}
	\end{subfigure}
	\hspace{10pt} %%
	\begin{subfigure}[b]{0.4\columnwidth}
		\includegraphics[width=1.25\linewidth]{figures/slack_distance32.png}
		%\caption{Picture 2}
		\label{fig:2}
	\end{subfigure}
\vspace{-10pt}
\caption{\small Slack $\lambda_2$ and minimum separation over time for 
two different 
initial conditions after the random sequence scheme.}
\label{fig:slackbad}
\end{figure}

The condition of Theorem \ref{th:CAMPC_success} could be violated but two UAS could still be separated by more than $\delta$m. This could happen because at the time step $k$ the separation between the two UAS is achieved through some other relative position configurations ($i$ in eq. \ref{eq:pickaside}) compared to the one that is used as a constraint in the optimization. At the time steps $k$ where the robustness tubes of the two UAS are themselves more than $\delta$m apart, having a $\lambda_{2,k}>0$ cannot result in a violation of eq. \ref{eq:msep}. Fig. \ref{fig:slackbad} shows a couple of such examples.

\subsection{Additional Resources}
\label{sec:crazyflie_appendix}
Videos of additional experimental recordings and simulations can be found at \url{https://tinyurl.com/yxttq7l5}

%
%\begin{figure}[tb]
%	\begin{center}
%		\includegraphics[width=0.45\textwidth]{placeholder.pdf}
%	\end{center}
%	{\footnotesize
%		\caption{Experimental setup with to Crazyflie drones representing UAS1 and UAS2}
%		\label{fig:crazyflie_setup}}
%\end{figure} 
\begin{figure}[tb]
	\begin{center}
		\includegraphics[width=0.45\textwidth]{figures/scenario1_wo_ca_traj_plot.png}
	\end{center}
	{\footnotesize
		\caption{\small Conflicting trajectories at halfway-point for 
		2 crazyflie quad-rotors. The 2 drones are unable to complete 
		the mission due to the collision at the conflicting point. 
		Video recordings of actual flight and tracking can be found 
		at \url{https://youtu.be/1YOO-vOh6Zg}, 
		\url{https://youtu.be/Of3EIwCGCrk}}
		\label{fig:scen1_wo_ca}}
\end{figure}
