# Supplementary material for: Learning-to-Fly: Learning-based Collision Avoidance for Scalable Urban Air Mobility
Source: arXiv:2006.13267 source file (2020-06-23)
Supplement: Supplementary file 2 [file crazy_exp_appendix.tex]

\subsection{Additional Resources}
\label{sec:crazyflie_appendix}
Videos of additional experimental recordings and simulations can be found at \url{https://tinyurl.com/yxttq7l5}

%
%\begin{figure}[tb]
%	\begin{center}
%		\includegraphics[width=0.45\textwidth]{placeholder.pdf}
%	\end{center}
%	{\footnotesize
%		\caption{Experimental setup with to Crazyflie drones representing UAS1 and UAS2}
%		\label{fig:crazyflie_setup}}
%\end{figure} 
\begin{figure}[tb]
	\begin{center}
		\includegraphics[width=0.45\textwidth]{figures/scenario1_wo_ca_traj_plot.png}
	\end{center}
	{\footnotesize
		\caption{\small Conflicting trajectories at halfway-point for 
		2 crazyflie quad-rotors. The 2 drones are unable to complete 
		the mission due to the collision at the conflicting point. 
		Video recordings of actual flight and tracking can be found 
		at \url{https://youtu.be/1YOO-vOh6Zg}, 
		\url{https://youtu.be/Of3EIwCGCrk}}
		\label{fig:scen1_wo_ca}}
\end{figure}
