# Supplementary material for: Learning-to-Fly: Learning-based Collision Avoidance for Scalable Urban Air Mobility
Source: arXiv:2006.13267 source file (2020-06-23)
Supplement: Supplementary file 3 [file greedyAlgo.tex]

\subsection{A greedy algorithm for conflict resolution}
\label{sec:greedy_alg}

For a horizon length of $N$ steps, there are $6^{N}$ possible selections for the deconfliction constraints $H^i_k, \, g^i_k$ (6 at each time step in the horizon). The centralized MILP formulation picks which constraint to use by activating the corresponding binary variable \eqref{eq:CentralMILP}. For CA-MPC, we need a decision making algorithm to pick these constraints as there are no binary variables in the CA-MPC formulations \eqref{eq:drone1mpc}, \eqref{eq:drone2mpc}. 

The following is a greedy approach to this:

\begin{algorithm}
 \KwData{Pre-planned trajectories: $\mathbf{x_1}, \, \mathbf{x_2}$, a preset maneuver: $\text{preset} \in \{1,\dotsc,6\}$}
 \KwResult{$d_k \in \{1,\dotsc,6\}\, \forall k=\{0,\dotsc, N+1\}$ for conflict resolution maneuvers $H^{d_k},\, g^{d_k}$}
 initialization k=0, \; \\
 \While{$k \leq N+1$}{
 \For{$i=\{1,\dotsc,6\}$}
 {$r^{i}_k = g^i - H^i C(x_{1,k}-x_{2,k})$
 }
 %$i[k] = \text{argmax}_i\, (g_i - H_i (x_1[k]-x_2[k]))$ \\
 \eIf{$\exists i|r^i_k \geq 0 $}{
 $d_k = \text{argmax}_i\, r_{i}[k]$
 }
 {$d_k = \text{preset}$
 }
 k = k+1
%  read current\;
%  \eIf{understand}{
%   go to next section\;
%   current section becomes this one\;
%   }{
%   go back to the beginning of current section\;
%  }
 }
 \caption{Greedy conflict resolution}
 \label{alg:greedy}
\end{algorithm}

Algorithm \ref{alg:greedy}, for time steps $k$ such that there is no 
conflict, selects the direction (or side of the hypercube 
\eqref{eq:noconf}) where there is the most separation between the 
UAS. For the time steps where there is a conflict, it picks a 
pre-defined maneuver.
