# Supplementary material for: Learning-to-Fly: Learning-based Collision Avoidance for Scalable Urban Air Mobility
Source: arXiv:2006.13267 source file (2020-06-23)
Supplement: Supplementary file 4 [file rural_case.tex]

\subsection{Case Study: Equipment Surveillance Scenario}
\label{sec:rural_case}

\begin{figure}[tb]
	\begin{center}
		\includegraphics[width=0.49\textwidth]{figures/rural_out}
	\end{center}
	{\footnotesize
		\caption{\small Trajectories for 4 UAS tasked with flying over the
			pumpjacks by reaching the all green-colored goal set 
			within 10 minutes, while avoiding the all black-colored 
			obstacles (the
			pumpjacks themselves).}
		\label{fig:rural}}
\end{figure}

The equipment surveillance scenario taken 
from~\cite{wargo2014unmanned} outlines a low-altitude mission profile 
for four UAS operating within a sparsely populated area. The airspace 
setting is depicted in a Figure~\ref{fig:rural}. This scenario can 
serve as a template
for other rural use cases for UAS such as end-point package
deliveries and wildfire management.

The mission for each UAS $j\in\{1,\ldots,4\}$
is formalized in STL as following:
\begin{equation}
\label{eq:rural_d}
\begin{aligned}
\varphi_j =  \bigwedge_{n=1}^5
\eventually_{[0,10]} (p_j \in \text{Zone}_n)
&\land \eventually_{[9,10]} (p_j \in \text{EndZone}_j) \\
&\land\always_{[0,10]} \neg (p_j \in \text{Unsafe})
\end{aligned}
\end{equation}
where 
$T=10$m is the maximum allowable flight time
allocated to the mission, $\text{Zone}_n$ denotes the airspace region 
directly above each
of the five pumpjacks, $\text{Unsafe}$ denotes the no-fly zones within
the mission environment and $\text{EndZone}_j$ defines the region 
signifying the end of the UAS mission.

Table~\ref{tbl:runtimes_rural} shows the computation times 
for solving the planning problem in a centralized manner versus 
solving for each 
UAS $j$ and its specification $\varphi_j$ separately.

\begin{table}[]
	
	\caption{Computation times for the centralized versus individual 
		UAS planning
	}
	\label{tbl:runtimes_rural}
	
	\centering
	\begin{tabular}{c|c|c|c|c|c|}
		\cline{2-6}
		\multicolumn{1}{l|}{}                   & 
		\textbf{Centralized} & 
		\multicolumn{4}{c|}{\textbf{Independent 
				planning}}                   
		\\ \cline{2-6} 
		& \textbf{4 UAS}    & \textbf{UAS 1} & \textbf{UAS 2} & 
		\textbf{UAS 3} & \textbf{UAS 4} \\ \cline{2-6} 
		\hline\hline
		\multicolumn{1}{|c|}{\textbf{Mean (s)}} & 
		81.918               & 15.596          & 
		17.444            & 
		17.553           &   16.128        \\ \hline
		\multicolumn{1}{|c|}{\textbf{SD (s)}} & 
		27.215           & 6.257        & 
		7.404            & 
		6.912           &  6.764        \\ \hline
	\end{tabular}
\end{table}
