# Supplementary material for: Learning-to-Fly: Learning-based Collision Avoidance for Scalable Urban Air Mobility
Source: arXiv:2006.13267 source file (2020-06-23)
Supplement: Supplementary file 5 [file separation.tex]

\subsection{Separation Profile}
\label{sec:separation}

Figure~\ref{fig:sep_profile} depicts the separation profile over 
time before and after L2F for one of 10K minimum-jerk random 
trajectories described in the Section~\ref{sec:exp_setup}.

\begin{figure}[t]
	\begin{center}
		\includegraphics[width=0.45\textwidth]{figures/t3.png}
	\end{center}
	{\footnotesize
		\caption{\small The separation profile before and after L2F 
		for one of the minimum-jerk random trajectories described in 
		the Section~\ref{sec:exp_setup}.}
		\label{fig:sep_profile}}
\end{figure}
