# Supplementary material for: Learning-to-Fly: Learning-based Collision Avoidance for Scalable Urban Air Mobility
Source: arXiv:2006.13267 source file (2020-06-23)
Supplement: Supplementary file 6 [file slack-separation.tex]

\subsection{Brief discussion on minimum separation and CA-MPC 
objective value}
\label{sec:slackbad}

\begin{figure}
	\begin{subfigure}[b]{0.4\columnwidth}
		\includegraphics[width=1.25\linewidth]{figures/slack_distance153.png}
		%\caption{Picture 1}
		\label{fig:1}
	\end{subfigure}
	\hspace{10pt} %%
	\begin{subfigure}[b]{0.4\columnwidth}
		\includegraphics[width=1.25\linewidth]{figures/slack_distance32.png}
		%\caption{Picture 2}
		\label{fig:2}
	\end{subfigure}
\vspace{-10pt}
\caption{\small Slack $\lambda_2$ and minimum separation over time for 
two different 
initial conditions after the random sequence scheme.}
\label{fig:slackbad}
\end{figure}

The condition of Theorem \ref{th:CAMPC_success} could be violated but two UAS could still be separated by more than $\delta$m. This could happen because at the time step $k$ the separation between the two UAS is achieved through some other relative position configurations ($i$ in eq. \ref{eq:pickaside}) compared to the one that is used as a constraint in the optimization. At the time steps $k$ where the robustness tubes of the two UAS are themselves more than $\delta$m apart, having a $\lambda_{2,k}>0$ cannot result in a violation of eq. \ref{eq:msep}. Fig. \ref{fig:slackbad} shows a couple of such examples.
